# Supplementary material for: DeepView: Visualizing Classification Boundaries of Deep Neural Networks as Scatter Plots Using Discriminative Dimensionality Reduction
Source: arXiv:1909.09154 source file (2020-08-19)
Supplement: Supplementary file 1 [file suppl1.tex]

\begin{lemma}
    Let $S$ be a finite dimensional real vector space. Let $d : S \times S \to \R$ be a metric induced by an inner product and $X$ be a $S$-valued random variable. Then it holds
    \begin{align*}
    \argmin_{x \in S} \E\left[ d(X,x)^2 \right] &= \argmin_{x \in S} \E\left[ \Vert X - x \Vert_2^2 \right].
    \end{align*}
    \begin{proof}
        Since $d$ is induced by an inner product we may find a matrix $A$ such that $d(x,y)^2 = (x-y)^tA(x-y)$. 
        
        \textbf{1. Case $A$ is a diagonal matrix: } Then it holds
        \begin{align*}
        \E\left[ d(X,x)^2 \right] &= \sum_i a_{ii} \E\left[(X_i - x_i)^2\right]
        \end{align*}
        since we may optimize each component of $x$ separately the statement follows.
        
        \textbf{2. Case $A$ is not diagonal: } Using the spectral theorem we obtain $A = U^tDU$ (by spectral theorem we obtain $A = VDV^t$ then we define $U = V^t$, since $V$ is unitary so is $U$), where $D$ is a diagonal matrix an $U$ is unitary. Hence it follows
        \begin{align*}
        \argmin_{x \in S} \E\left[ d(X,x)^2 \right] 
        &=\argmin_{x \in S} \E\left[ (U(X-x))^tD(U(X-x)) \right] 
        \\&=\argmin_{x \in S} \E\left[ (UX-Ux)^tD(UX-Ux) \right] 
        \\&=U^{-1} \argmin_{x' \in \im U} \E\left[ (UX-x')^tD(UX-x') \right] 
        \\&=U^{-1}\argmin_{x' \in \im U} \E\left[ \Vert UX - x'\Vert_2^2 \right] & \text{1. Case}
        \\&=\argmin_{x \in S} \E\left[ \Vert UX-Ux \Vert_2^2 \right] 
        \\&=\argmin_{x \in S} \E\left[ \Vert U(X-x) \Vert_2^2 \right] 
        \\&=\argmin_{x \in S} \E\left[ \Vert X-x\Vert_2^2 \right]. & \text{$U$ is unitary}
        \end{align*}
    \end{proof}
\end{lemma}

\begin{remark}[Derivation of $\piinv$]
It holds
\begin{align*}
\piinv(\y) &:= \argmin_{\x \in S} \sum_{i = 1}^n D(p_i(\y)||q_i(\x)) \overset{!}{=} \argmin_{\x \in S} \sum_{i = 1}^n H(p_i(\y);q_i(\x)) 
\end{align*}
since $\frac{\partial}{\partial \theta} D_\KL (X \Vert f_\theta(Y) ) = \frac{\partial}{\partial \theta} (H(X ; f_\theta(Y)) - H(X)) = \frac{\partial}{\partial \theta} H(X ; f_\theta(Y))$, where $H(\cdot)$ denotes entropy and $H(\cdot;\cdot)$ denotes the cross entropy. Now by plugging in the definitions and approximations we obtain
\begin{align*}
H(\y;\x) &= -\sum_{i = 1}^n w_i(\y) \log v_i(\x) \underbrace{-\sum_{i = 1}^n (1-w_i(\y))\log (1-v_i(\x))}_{\approx 0} \\&= -\sum_{i = 1}^n w_i(\y) \left(- \frac{\Vert \x - \s_i \Vert_2^2}{\sigma_i} \right) \\&= \sum_{i = 1}^n \frac{w_i(\y)}{\sigma_i} \Vert \x -  \s_i \Vert_2^2 
\\\Rightarrow \nabla_\x H(\y;\x) &= 2 \sum_{i = 1}^n \frac{w_i(\y)}{\sigma_i} (\x - \s_i) \overset{!}{=} 0
\\\Leftrightarrow \x &= \frac{\sum_{i = 1}^n \frac{w_i(\y)}{\sigma_i} \s_i }{\sum_{i = 1}^n \frac{w_i(\y)}{\sigma_i}}.
\end{align*}
Furthermore using the lemma above we see that
\begin{align*}
    \x^*
      &= \argmin_{\x \in S} -\sum_{i = 1}^n w_i(\y) \log v_i(\x) 
    \approx \argmin_{\x \in S} \sum_{i = 1}^n \frac{w_i(\y)}{\sigma_i} d_{s^*}(\x,\s_i)^2
    \\&= \argmin_{\x \in S} C \sum_{i = 1}^n \frac{\frac{w_i(\y)}{\sigma_i}}{C} d_{s^*}(\x,\s_i)^2
    = \argmin_{\x \in S} C \E_P[ d_{s^*}(\x,X)^2 ]
    \\&= \argmin_{\x \in S} C \E_P[ \Vert \x - X \Vert^2 ]
    =\argmin_{\x \in S} C \sum_{i = 1}^n \frac{\frac{w_i(\y)}{\sigma_i}}{C} \Vert \x - \s_i \Vert^2
    \\&= \frac{\sum_{i = 1}^n\frac{w_i(\y) \s_i}{\sigma_i}}{\sum_{i = 1}^n\frac{w_i(\y)}{\sigma_i}},
\end{align*}
where $C = \sum_{i = 1}^n\frac{w_i(\y)}{\sigma_i}$, $d_{s^*}$ the approximation of $d_S$ at ${s^*}$, $X : \{1,...,n\} \to , i \mapsto \s_i$ a random variable and $P(I) = \frac{1}{C} \sum_{i \in I} \frac{w_i(\y)}{\sigma_i}$.
\end{remark}

\begin{lemma}[Derivation of $\eta_\textnormal{opt}$]
Let $R,S$ be finite dimensional, real vector spaces. Let $\r_i \in R,\s_i \in S,A_i \in \textnormal{Mat}_\R(S,S), \; i = 1,...,n$ and $\Theta,J \in \textnormal{Mat}_\R(R,S)$. Assume that $A_i$ are symmetric and positive definite and denote by $\Vert \cdot \Vert_i$ the induced norm, i.e. $\Vert s \Vert_i := \sqrt{s^t A_i s}$. Then it holds
\begin{align*}
\argmin_{\eta} \sum_{i = 1}^n \Vert (\Theta-\eta J) \r_i - \s_i \Vert_i^2 = \frac{\sum_{i = 1}^n (\Theta \r_i - \s_i)^t A_i J \r_i }{\sum_{i = 1}^n \r_i^t J^t A_i J \r_i }.
\end{align*}
\begin{proof}
It holds
\begin{align*}
\frac{\d}{\d \eta} \sum_{i = 1}^n \Vert (\Theta-\eta J) \r_i - \s_i \Vert_i^2 
&= 2 \sum_{i = 1}^n ((\Theta-\eta J) \r_i - \s_i)^t A_i J \r_i \overset{!}{=} 0 \\
\Leftrightarrow \sum_{i = 1}^n (\Theta \r_i - \s_i)^t A_i J \r_i &= \eta \sum_{i = 1}^n \r_i^t J^t A_i J \r_i
\end{align*}
\end{proof}
\end{lemma}

\begin{algorithm}
    \caption{Construction of Delaunay neighborhood}
    \label{ConstTriaN}
    \begin{algorithmic}[1]
        \Procedure{ConstructDelaunayNeighborhood}{$(r_i)_{i=1,...,n}$ data points, $n_s$ number of simplices, $n_k$ number of neighbors, $\varepsilon$ minimal border distance}
        \State $C \gets \Call{K-Means}{(r_i)_i,n_s}$\;
        \State $B \gets \Call{Border}{(r_i)_i, \varepsilon}$\;
        \Comment{Vertices of a rectangle containing $\cup_i B_{r_i}(\varepsilon)$}
        \State $V \gets C \cup B$\;
        \Comment{Assure that every $r_i$ is actually contained in one simplex}
        \State $S \gets \Call{DelaunayTriangulation}{V}$\;
        \Comment{Delaunay triangulation for $V$, returns set of simplices}
        \For{$i \in [1,|S|]_\N$}
        \State $V' \gets \Call{GetVertices}{S_i}$\;
        \Comment{Vertices of $S_i$} 
        \For{$j \in [1,D+1]_\N$}
        \State $\nu_j \gets \Call{NearestNeighbors}{(r_i)_i, V'_j, n_k}$\;
        \Comment{$n_k$ nearest neighbors of $V'_j$ in $(r_i)_i$ sorted by distance}
        \EndFor
        \State $N_i \gets \Call{ComposeNeighbors}{\nu , n_k}$
        \EndFor
        \State \textbf{return} $S, N$ 
        \Comment{Delaunay triangulation $S$, Delaunay neighborhood $N$}
        \EndProcedure
        
        \Procedure{ComposeNeighbors}{$(N_{ij})_{i=1,...,n,\;j=1,...,n_k}$ 2d-array of nearest neighbors; row wise sorted by distance, $n_k$ number of neighbors}
        \For{$i \in [1,n]_\N$}
        \State $k_i \gets 0$ 
        \EndFor
        \State $D \gets \emptyset$ \;
        \Comment{Use a heap for speedup}
        \State $j \gets 1$\;
        \State $i \gets 1$ \;
        \While{$j \leq n_k$}
        \State $k_i \gets k_i +1$ \;
        \If{$N_{ik_i} \not\in D$}
        \Comment{$N_{ik_i}$ is not already contained in $C$}
        \State $D \gets D \cup \{N_{ik_i}\}$\;
        \State $C_j \gets N_{ik_i}$ \;
        \State $i \gets (i \mod n)+1$ \;
        \State $j \gets j+1$ \;
        \EndIf
        \EndWhile
        \State \textbf{return} $C$ 
        \Comment{composed neighborhood}
        \EndProcedure   
    \end{algorithmic}
\end{algorithm}
