# Supplementary material for: DeepView: Visualizing Classification Boundaries of Deep Neural Networks as Scatter Plots Using Discriminative Dimensionality Reduction
Source: arXiv:1909.09154 source file (2020-08-19)
Supplement: Supplementary file 2 [file suppl2.tex]

\begin{figure}
  \centering
  \includegraphics[width=0.49\linewidth]{imagenet_classifVis_annotated}
  \includegraphics[width=0.5\linewidth, trim= 0mm 0mm 0mm 0mm]{imagenet_invExamples}
  \caption{A visualization of a part of ImageNet and the AlexNet network together with markers of specified positions around the adversarial example (left). The resulting images of the inverse mapping $\piinv$ for the previously specified positions, together with the assigned label and according certainty of the classifier (right).}
  \label{fig:imagenet}
\end{figure}

For our current experiments we utilize a subset of three classes from the full ImageNet data set,\footnote{http://image-net.org/} the classes 'acoustic guitar', 'electric guitar' and 'grand piano'. 
As the pre-trained model we choose the popular AlexNet \cite{alexnet} and apply DeepView to 300 randomly selected data points and one adversarial example. 

The resulting visualization is shown in \fig\ \ref{fig:imagenet} with additional white circles around points for which the $\piinv$ mapping is inaccurate (i.e.\ where $\Qd$ counts mistakes). The evaluation is summarized in \tab\ \ref{tab:eval_res} and reveals lower scores as compared to the CIFAR-10 dataset. This is not surprising because the dataset, as well as the classifier (being trained on 1000 classes), is much more complex. Furthermore, the scores do not consider a top-5 measure as partially common with this dataset.

Concerning the visualization, we can observe that the 'piano' class is further away from the other two and that a set of points is classified as 'other' and is positioned in the middle. 
Again, the adversarial example is positioned outside of the main cluster and we investigate the area around it in the same as previously. While the position '0' is mapped to an image which is classified properly, the images of '1' to '5' are predicted with a high uncertainly and partially even wrong, although showing clearly guitars. 

We select two further areas close to points being outside of their main cluster and mark them with '6' and '7'. This way we can get an impression why these images are classified incorrectly. In this case, the images show multiple objects with the target object being partially rather in the background.
